# Supplementary material for: Metastability as a mechanism for yielding in amorphous solids under cyclic shear
Source: arXiv:2106.13069 ancillary file (2021-12-13)
Supplement: Supplementary file 1 [file SupplementalMaterial.pdf]

# Supplemental Material to "Metastability as a mechanism for yielding in amorphous solids under cyclic shear"

Muhittin Mungan[1,*] and Srikanth Sastry[2,†]

[1] *Institut für angewandte Mathematik, Universität Bonn, Endenicher Allee 60, 53115 Bonn, Germany*
[2] *Jawaharlal Nehru Centre for Advanced Scientific Research, Jakkar Campus, 560064 Bengaluru, India*

## I. OUTLINE

The supplemental material is organized as follows. We review in Section II the potential-theoretical approach to metastability for calculating expected hitting/first-passage times of Markov Chains with a finite state space. We then specialize to the case when the Markov Chain describes a one-dimensional nearest-neighbour random walk and derive the well-known expression for the first-passage times, Eqs. (4) and (5) of the main text. This section is optional and can be skipped. Its main purpose is to give a self-contained presentation of the potential-theoretical approach to metastability that is accessible to a physics audience. In Section III, we then work out the expected first-passage time $\tau_{\rm abs}(\gamma)$ for the Ehrenfest model, Eq. (6) of the main text. Here we also describe the continuum limit of the dynamics, which is governed by a Fokker-Planck equation. In Section IV we calculate the yielding point of the Ehrenfest Model to leading order, providing a derivation of Eq. (8) of the main text, and work out higher order corrections. In Section V we give further details on the two activation processes described in the main text, as a result of which the dynamics of the Ehrenfest model can transition back from its absorbing region into the steady-state regime. We consider first the dynamics with a fixed activation rate, and then the general case where activated dynamics within the whole absorbing region can occur.

## II. THE POTENTIAL THEORETICAL APPROACH TO HITTING TIMES AND METASTABILITY

In the following three subsections we review the general framework for calculating the hitting times of a reversible Markov chain and then work these out in the next section for the special case of the Ehrenfest trap model. We restrict the discussion to time-homogeneous Markov chains in discrete time and on a finite state space $\mathcal{S}$. The treatment presented here is based on the potential theoretical approach to metastability, as initiated in a 2001 paper by Bovier, Eckhoff, Gayrard and Klein [1] and expounded in the recent monograph by Bovier and den Hollander [2]. Here we will follow very closely the treatment of [2], where further details can be found. Our main purpose is to give a self-contained treatment of the main ingredients of this approach. For the basic theory of Markov chains, we refer the reader to the mongraph by Norris [3].

### A. Expected hitting times as solutions to boundary value problems

For $n \in \mathbb{N}_0$, we denote by $X_n, X_{n+1} \in \mathcal{S}$ the states of the Markov chain at times $n$ and $n+1$. The transition probability is then given as

$$\mathbb{P}(X_{n+1} = y | X_n = x) = p(x,y), \tag{1}$$

where by time-homogeneity the transition probability does not depend on $n$. Note that for purposes of familiarity we have followed a physics-style notation in the main text. However, in order to facilitate comparison with the results in [2], we will use the notation developed there. When we turn to the discussion of the Ehrenfest model and its first-passage time in Section III, we will re-express these results in the notation of the main text.

We further assume that the Markov chain is *irreducible*, so that for each pair of states $x, y \in \mathcal{S}$ there exists some times $n, m$ such that $\mathbb{P}(X_n = y | X_0 = x) > 0$ and $\mathbb{P}(X_m = x | X_0 = y) > 0$. For a finite state space $\mathcal{S}$, irreducibility implies that there exists a unique invariant measure $\mu(x)$ [3], so that

$$\mu(x) = \sum_{y \in \mathcal{S}} \mu(y)\, p(y,x) \equiv (\mu p)(x). \tag{2}$$

It is useful to introduce the *generator* of the Markov process as

$$L(x,y) = p(x,y) - \delta_x(y), \tag{3}$$

where $\delta_x(y)$ is the Kronecker-delta. The invariant measure thus satisfies

$$(\mu L)(x) = 0. \tag{4}$$

An irreducible Markov chain is said to be *reversible*, if it obeys the *detailed-balance conditions*:

$$\mu(x) p(x,y) = \mu(y) p(y,x), \tag{5}$$

for each pair of states $x, y \in \mathcal{S}$.

* Corresponding author: mungan@iam.uni-bonn.de
† Corresponding author: sastry@jncasr.ac.in

Given an initial state $X_0 = x$ and a subset $A$ of $\mathcal{S}$, we are interested in the *hitting time* $\tau_A$ of the set $A$, defined as

$$\tau_A = \min\left(n > 0 \,:\, X_n \in A\right). \tag{6}$$

Note that $\tau_A$ is the first time the system reaches the set $A$ *after* initialization, and regardless of whether the Markov chain was initialized in $A$ or not.

In the remainder we will only be considering Markov chains initialized in some state $X_0 = x$. We will then write then probabilities or expectations conditioned on the event $X_0 = x$ as $\mathbb{P}_x$, respectively $\mathbb{E}_x$.

Given a pair of disjoint subsets $A, B \subset \mathcal{S}$, we consider next the probability $\mathbb{P}_x(\tau_A < \tau_B)$ that a Markov chain initialized at $x$ reaches the set $A$ before $B$. For $x \notin A \cup B$, this probability turns out to be given by

$$\mathbb{P}_x(\tau_A < \tau_B) = h_{A,B}(x), \tag{7}$$

where $h_{A,B}(x)$ is the solution of the following (discrete) boundary value problem:

$$(Lh_{A,B})(x) = 0, \quad x \notin A \cup B, \tag{8}$$

$$h_{A,B}(x) = 1, \quad x \in A, \tag{9}$$

$$h_{A,B}(x) = 0, \quad x \in B, \tag{10}$$

where $(Lh_{A,B})_x \equiv \sum_y L(x,y) h_{A,B}(y)$. To see this, regard (9) and (10) as definitions of $h_{A,B}$ in $A \cup B$ and note that for $x \notin A \cup B$, the first transition is either into the state $A$, or into some other state so that

$$\mathbb{P}_x(\tau_A < \tau_B) = \sum_{y \in A} p(x,y) + \sum_{y \in (A \cup B)^c} p(x,y) \mathbb{P}_y(\tau_A < \tau_B). \tag{11}$$

Using the definition of the generator (3), the above equation then reduces to (8). The cases where $x$ is initially in $A$ or $B$ are treated by a similar line of reasoning and one finds that

$$\mathbb{P}_x(\tau_A < \tau_B) = \begin{cases} h_{A,B}(x), & x \notin A \cup B, \\ -e_{A,B}(x), & x \in B, \\ 1 - e_{A,B}(x), & x \in A, \end{cases} \tag{12}$$

where

$$e_{A,B}(x) = (-Lh_{A,B})(x) = -\sum_{y \in \mathcal{S}} L(x,y) h_{A,B}(y), \tag{13}$$

is called the *equilibrium measure*.

As we shall see shortly, the family of solutions $h_{A,B}$ parametrized by the pairs of disjoint sets $A$ and $B$, is key in the calculation of various statistics related to hitting times. It is called the *equilibrium potential*, since the discrete boundary value problem (8) – (10) emerges naturally in the case of networks of resistors or capacitors in which a subset $A$ of the vertices is kept at unit potential 1, while another subset $B$ is grounded. Then, (8) corresponds to the Kirchhoff rule for the node $x$ whose potential has not been assigned by the boundary conditions. The components of $L$ can therefore be interpreted as conductances, or in the case of a network of capacitors as capacitances. This interpretation should not be taken too literally, since the "circuit elements" in question have a polarity, *i.e.* $p(x,y) \neq p(y,x)$ in general. Nevertheless, the analogy with electrical circuits already suggest that the solution of the boundary value problem (8) – (10) can be cast as the solution of a variational problem, namely assigning the potentials at the remaining vertices in such a way that an energy-like functional of the network is minimized. The power of the potential theoretical approach lies in the fact that it is often easier to come up with functions that approximately minimize the variational functional, which often provide rather good approximate solutions to the boundary value problem.

We consider next the expected time $\mathbb{E}_x(\tau_B)$ to reach a set $B \subset \mathcal{S}$, given that the Markov chain was initialized in a state $X_0 = x$. Assuming again first that $x \notin B$, a similar reasoning that led to (11) gives

$$\mathbb{E}_x(\tau_B) = \sum_{y \in B} p(x,y) + \sum_{y \in B^c} p(x,y)\left[1 + \mathbb{E}_y(\tau_B)\right]. \tag{14}$$

Defining

$$w_B(x) = \begin{cases} \mathbb{E}_x(\tau_B), & x \notin B, \\ 0, & x \in B, \end{cases} \tag{15}$$

from (14) it is found that $w_B(x)$ satisfies the following boundary value problem:

$$(-Lw_B)(x) = 1, \quad x \notin B, \tag{16}$$

$$w_B(x) = 0, \quad x \in B. \tag{17}$$

One can then show that

$$\mathbb{E}_x(\tau_B) = \begin{cases} w_B(x), & x \notin B, \\ 1 + (Lw_B)(x), & x \in B. \end{cases} \tag{18}$$

Comparing the two boundary value problems (8) – (10) and (16) – (17), we see that they both prescribe a function that vanishes on the (non-empty) set $B$. Treating the set $B$ as fixed, it turns out [2, 3] that the generator $L$ is invertible on $B^c$, furnishing thereby the Green's function $G_B(x,y)$ for the inhomogeneous boundary value problem (16) – (17). We define $G_B$ such that $(G_B L)(x,y) = -\delta_x(y)$ for all $x, y \in B^c$. Assuming now that the boundary value problem (8) – (10) has been solved for arbitrary singleton sets $A = \{z\} \subset B^c$, so that $h_{\{z\},B}(x)$ is known for all $x, z \in B^c$, we can express $G_B$ in terms of the equilibrium potentials as

$$G_B(x,z) = \frac{h_{z,B}(x)}{e_{z,B}(z)}, \tag{19}$$

where $e_{z,B}(z) = -(Lh_{z,B})(z)$, *cf.* (13), and we henceforth drop curly braces around singleton sets.

Thus for $x \notin B$ we obtain the expected hitting time $\mathbb{E}_x(\tau_B)$ of the set $B$ as

$$\mathbb{E}_x(\tau_B) = \sum_{z \in B^c} G_B(x,z) = \sum_{z \in B^c} \frac{h_{z,B}(x)}{e_{z,B}(z)}. \tag{20}$$

In the case that the reversible Markov chain describes a one-dimensional nearest-neighbour random walk, as is the case of the Ehrenfest trap model, the bounday value problem (8) – (10) can be solved explicitly, and we turn next to it.

### B. The $1d$ nearest-neighbour random walk

The treatment presented here again follows closely that of [2]. We shall assume that the state space is $\mathcal{S} = \{k\Delta : k = 0, 1, \ldots 2\mathcal{N}\}$, where $\Delta > 0$ is some spacing that we retain for book-keeping purposes. The condition of reversibility becomes

$$\mu(x)p(x, x+\Delta) = \mu(x+\Delta)p(x+\Delta, x), \tag{21}$$

for all $x \in \mathcal{S}$. Note that the nearest-neighbour nature of the transitions implies that the invariant measure can be inferred easily from the transition probabilities.

The generator of the Markov chain then becomes

$$\begin{aligned} L(x,y) = & \, p(x, x+\Delta)\delta_{x+\Delta}(y) + p(x, x-\Delta)\delta_{x-\Delta}(y) \\ & - (1 - p(x,x))\delta_x(y), \end{aligned} \tag{22}$$

which, using $p(x,x) = 1 - p(x, x+\Delta) - p(x, x-\Delta)$, can be re-expressed as

$$\begin{aligned} L(x,y) = & \, p(x, x+\Delta)\left(\delta_{x+\Delta}(y) - \delta_x(y)\right) \\ & + p(x, x-\Delta)\left(\delta_{x-\Delta}(y) - \delta_x(y)\right). \end{aligned} \tag{23}$$

We next consider a pair of states $a, b \in \mathcal{S}$ with $a < b$, and define the sets $B = \{x \geq b\}$ and $A = \{x \leq a\}$. Turning now to the boundary value problem (8) – (10) defined by the sets $A$ and $B$, we seek a solution $h(x) = h_{a,b}(x)$ for $a < x < b$ such that, *cf.* (8),

$$\begin{aligned} & p(x, x+\Delta)\left[h(x+\Delta) - h(x)\right] \\ & \quad + p(x, x-\Delta)\left[h(x-\Delta) - h(x)\right] = 0, \end{aligned} \tag{24}$$

subject to the boundary conditions $h(b) = 0$ and $h(a) = 1$. The solution of the recursion (24) is readily worked out. Defining the auxiliary variables

$$d(x) = h(x) - h(x-\Delta), \tag{25}$$

the recursion (24) becomes

$$p(x, x+\Delta)d(x+\Delta) - p(x, x-\Delta)d(x) = 0, \tag{26}$$

which is solved as

$$d(x) = \prod_{x \leq z < b} \frac{p(z, z+\Delta)}{p(z, z-\Delta)}\, d(b). \tag{27}$$

Applying now the reversibility condition (21), the product telescopes out, so that we are left only with the first and last factor,

$$d(x) = \frac{\mu(b)}{\mu(x-\Delta)}\, \frac{p(b, b+\Delta)}{p(x-\Delta, x)}\, d(b). \tag{28}$$

Solving now the recursion (25), we finally obtain the solution of the boundary value problem for $a < x < b$ as

$$h_{a,b}(x) = \frac{\sum_{x \leq z < b} \frac{1}{\mu(z)\, p(z, z+\Delta)}}{\sum_{a \leq z < b} \frac{1}{\mu(z)\, p(z, z+\Delta)}} \equiv \frac{c(a,b)}{c(x,b)}, \tag{29}$$

where

$$\frac{1}{c(a,b)} = \sum_{a \leq z < b} \frac{1}{\mu(z)\, p(z, z+\Delta)} \tag{30}$$

is called the *capacitance* between $a$ and $b$, Eq. (5) of the main text.

We will also need the equilibrium measure (13), which written out becomes

$$\begin{aligned} e_{a,b}(x) = & -(Lh_{a,b})(x) = -p(x, x+\Delta)\left[h(x+\Delta) - h(x)\right] \\ & - p(x, x-\Delta)\left[h(x-\Delta) - h(x)\right]. \end{aligned} \tag{31}$$

Since $h_{a,b}(x)$ is the solution of the boundary value problem (8) – (10), it is now easily shown that the only non-zero elements of $e_{a,b}(x)$ occur at $x = a$ and $x = b$ and are given as

$$e_{a,b}(a) = \frac{c(a,b)}{\mu(a)}, \tag{32}$$

$$e_{a,b}(b) = -\frac{c(a,b)}{\mu(b)}. \tag{33}$$

Thus from (12) we find that

$$\mathbb{P}_x(\tau_a < \tau_b) = \begin{cases} 1 - \frac{c(a,b)}{\mu(a)}, & x = a, \\ \frac{c(a,b)}{c(x,b)}, & a < x < b, \\ \frac{c(a,b)}{\mu(b)}, & x = b. \end{cases} \tag{34}$$

We obtain next an expression for the expected hitting time $\mathbb{E}_x(\tau_b)$ for $x < b$. From (20) we have

$$\mathbb{E}_x(\tau_b) = \sum_{z < b} \frac{h_{z,b}(x)}{e_{z,b}(z)}. \tag{35}$$

Noting that $h_{z,b}(x) = 1$ for $z \geq x$, and using (29) and (32), we obtain

$$\mathbb{E}_x(\tau_b) = \frac{1}{c(x,b)} \sum_{z \leq x} \mu(z) + \sum_{x < z < b} \frac{\mu(z)}{c(z,b)}, \tag{36}$$

which is Eq. (4) of the main text.

### C. Emergence of metastability for the 1d random walk

As we have shown in the previous section, the problem of finding the hitting probabilities $\mathbb{P}_x(\tau_a < \tau_b)$, Eq. (34), and the expected hitting times $\mathbb{E}_x(\tau_b)$, Eq. (36), have been reduced to the calculation of capacitances defined in (30). Suppose now that the invariant measure of the process is such that $\mu(x)$ is concentrated in a single small region $\mathcal{M} \subset \mathcal{S}$, taking there values of order one, while outside that region $\mu$ is exponentially small. This means that the random walk spends most of its time within the region $\mathcal{M}$ with occasional excursions out of it. If we assume further that the transition probabilities remain of order one (they cannot be zero, since the Markov chain is irreducible), then for the capacity $c(a,b)$ such that $a \in \mathcal{M}$ and $b \in \mathcal{M}^c$, this implies that the sums on the right hand side of (30) are dominated by the terms near $b$.

To see the implication of this observation, let us suppose that the sums can be approximated by retaining only their largest terms and let us consider first the escape probability $\mathbb{P}_a(\tau_b < \tau_a)$, which in this approximation then becomes

$$\mathbb{P}_a(\tau_b < \tau_a) = \frac{\mu(b)}{\mu(a)}\, p(b, b-\Delta) \le \frac{\mu(b)}{\mu(a)}. \tag{37}$$

By assumption the fraction is exponentially small so that the escape to $b$ is a rare event. Now every time the system returns to $a$ without having reached $b$, it has the same exponentially small probability $\mathbb{P}_a(\tau_b < \tau_a)$ to make it to $b$ in the next excursion. By the Markov property these excursions are independent and thus the number of excursions until an escape occurs are geometrically distributed with parameter $\mathbb{P}_a(\tau_b < \tau_a)$, so that the expected number of excursions is $1/\mathbb{P}_a(\tau_b < \tau_a)$.

In the limit of a very small escape probability, we have metastability, *i.e.* there exist two well-separated time scales: (i) a small time scale $\mathbb{E}_a(\tau_a)$ that describes the average duration of an excursion from $a$ to $a$ without reaching $b$, and (ii) a much larger time scale $\mathbb{E}_a(\tau_b)$, the waiting time for the first successful excursion to $b$, given that initially the Markov chain is in $a$. In the limit that $\mathbb{E}_a(\tau_b) \gg \mathbb{E}_a(\tau_a)$, the geometrical distribution of (discrete) waiting times will be increasingly well approximated by a (continuous) exponential distribution with expected waiting time given by $\mathbb{E}_a(\tau_b)$. These arguments can be made rigorous and we refer the reader to [2] for details.

## III. THE EHRENFEST MODEL

We turn next to the random walk associated with the Ehrenfest model. Setting $\Delta = 1/(2\mathcal{N})$, the mesostate energy $\epsilon_k = k/(2\mathcal{N})$ of the Ehrenfest model becomes $\epsilon_k = x$. It is more convenient to work with $x$ we have

$$p(x,y) = (1-x)\ \delta_{x+\Delta}(y) + x\, \delta_{x-\Delta}(y) \tag{38}$$

The Markov chain is irreducible and its invariant measure is given by

$$\mu(x) = \binom{2\mathcal{N}}{k} \frac{1}{2^{2\mathcal{N}}}, \quad x = k\Delta. \tag{39}$$

as is readily verified. Furthermore, the Markov chain is reversible, as can be checked easily.

Observe now that in the limit of large $\mathcal{N}$ the invariant measure is sharply peaked around the state $x = \mathcal{N}\Delta$. In fact, approximating the binomial in (39) via Stirling's formula we find that

$$\mu(x) = \frac{1}{2}\frac{1}{\sqrt{\pi\mathcal{N}}}\ [x\,(1-x)]^{-\frac{1}{2}}\ e^{-2\mathcal{N}I(x)}, \tag{40}$$

where

$$I(z) = \ln 2 + z\ln z + (1-z)\ln(1-z), \tag{41}$$

which expanded around $z = 1/2$ to second order becomes

$$I(z) = 2\left(z - \frac{1}{2}\right)^2. \tag{42}$$

We now take as our starting point $x = 1/2$, where the invariant distribution $\mu$ has its peak, and for $b > x$ consider the hitting times $\tau_b$. From (34) and (36) we have,

$$\mathbb{P}_{1/2}(\tau_b < \tau_{1/2}) = 1 - \mathbb{P}_{1/2}(\tau_{1/2} < \tau_b) = \frac{c(1/2,b)}{\mu(1/2)}, \tag{43}$$

and

$$\mathbb{E}_{1/2}(\tau_b) = \frac{1}{c(1/2,b)}\sum_{z\le 1/2}\mu(z) + \sum_{1/2<z<b}\frac{\mu(z)}{c(z,b)}. \tag{44}$$

As discussed before, for $b$ sufficiently far away from the peak at $x = 1/2$ of $\mu$, the sums in the capacities $c(1/2,b)$ and $c(z,b)$ are dominated by the terms near $b$, which then can be evaluated asymptotically in $\mathcal{N}$ using Laplace's method. Consequently, asymptotically in $\mathcal{N}$ we have $c(1/2,b) \sim c(z,b)$, and hence $\mathbb{E}_{1/2}(\tau_b)$ simplifies as

$$\mathbb{E}_{1/2}(\tau_b) = \frac{1}{c(1/2,b)}. \tag{45}$$

We now derive the expression for the expected waiting time stated in the main text. Substituting the asymptotic expression (40) into (30) we obtain

$$\frac{1}{c(1/2,b)} = \sum_{1/2\le z<1/2} g\,(z)\ e^{2\mathcal{N}I(z)}, \tag{46}$$

where

$$g(z) = 2\sqrt{\pi\mathcal{N}\,\frac{z}{1-z}}. \tag{47}$$

Due to the prefactor $2\mathcal{N}$ in the exponential, which is large, and the fact that the function $I(z)$ is increasing in

$1/2 < z < b$, the exponential term drops rapidly when $z$ moves further away from for $b$. Therefore, for large $\mathcal{N}$, this sum is dominated by the terms near $b$. At the same time the pre-factor $g(z)$ changes slowly in this region and we can therefore replace $z$ in $g(z)$ by $b$, so that we obtain

$$\frac{1}{c(1/2,b)} = g\,(b) \sum_{1/2 \le z < b} e^{2\mathcal{N} I(z)}. \tag{48}$$

Letting now $b = k/(2\mathcal{N})$ and writing $z = b - j/(2\mathcal{N})$, we obtain

$$\frac{1}{c(1/2,b)} = g\,(b) \sum_{j=1}^{\mathcal{N}-k} e^{2\mathcal{N} I\left(b - \frac{j}{2\mathcal{N}}\right)}. \tag{49}$$

Since we are interested in an expression asymptotic in $\mathcal{N}$, we can carry out the summation by expanding $I$ around $b$ to first order and sum the resulting geometric series by letting the upper boundary go to infinity (which will only introduce a correction that is exponentially small). Thus we approximate the sum via the following steps

$$\begin{aligned} \sum_{j=1}^{\mathcal{N}-k} e^{2\mathcal{N} I\left(b - \frac{j}{2\mathcal{N}}\right)} &= e^{2\mathcal{N} I(b)} \sum_{j=1}^{\mathcal{N}-k} e^{-j\,I'(b)} \\ &= e^{2\mathcal{N} I(b)} \sum_{j=1}^{\infty} e^{-j\,I'(b)} \\ &= \frac{e^{-I'(b)}}{1 - e^{-I'(b)}}\, e^{2\mathcal{N} I(b)} \\ &= \frac{1-b}{2b-1}\, e^{2\mathcal{N} I(b)}, \end{aligned} \tag{50}$$

where in the last line we used (41).

Substituting (50) into (49), and using (47) and (45), we finally obtain

$$\mathbb{E}_{1/2}(\tau_b) = 2\sqrt{\pi\mathcal{N}}\,\sqrt{b(1-b)}\,\frac{e^{2\mathcal{N} I(b)}}{2b-1}, \tag{51}$$

where $b = k/2\mathcal{N} > 1/2$. Specifically, in the Ehrenfest model $b = \epsilon_\gamma$ marks the boundary of the absorbing region, and we recover Eq. (6) of the main text,

$$\tau_{\text{abs}}(\gamma) \equiv \mathbb{E}_{1/2}(\tau_{\epsilon_\gamma}) = 2\sqrt{\pi\mathcal{N}}\,\sqrt{\epsilon_\gamma(1-\epsilon_\gamma)}\,\frac{e^{2\mathcal{N} I(\epsilon_\gamma)}}{2\epsilon_\gamma - 1}. \tag{52}$$

Let us remark that Eq. (51) was derived in a slightly different setting by Bellman and Harris as Eq. (6) in [4], where our $b = k/(2\mathcal{N})$ and their $\lambda = k/\mathcal{N}$, so that the relation between these is $b/2 = \lambda$. Specifically, Bellman and Harris consider (i) the case $b < x$, and (ii) impose a continuous time dynamics for the transfer of balls between urns, such that the time between transfers is exponentially distributed with mean $1/\mathcal{N}$. Bellman and Harris result can be recovered from (51) (or *vice versa*) by accounting for these two differences as follows: (i) by exploiting the obvious symmetry around $x = 1/2$, and letting $b \to 1-b$ in (51), and (ii) by noting that the average time between transfers in their case is $1/\mathcal{N}$ and thus multiplying (51) by $1/\mathcal{N}$, which is permissible for $\mathcal{N}$ large and a large number of transfers.

### A. Continuum approximation via Fokker Planck equations

In the limit of large $\mathcal{N}$, such that $\Delta = 1/(2\mathcal{N})$, $\epsilon = k\Delta$, and a rescaling of time $t$ as $t = n\eta\Delta$, where $\eta$ sets a time scale, the dynamics of the Ehrenfest urns can be approximated by an Ornstein-Uhlenbeck process [5]. The probability density $P(\epsilon, t)$ that the system is in state $\epsilon$ at times $t$ then satisfies Smoluchowski's equation [5]

$$\frac{\partial P}{\partial t} = \frac{2}{\eta}\frac{\partial}{\partial \epsilon}\left(\left[\epsilon - \frac{1}{2}\right] P\right) + \frac{\Delta}{2\eta}\frac{\partial^2 P}{\partial \epsilon^2}, \tag{53}$$

where $\Delta/\eta$ furnishes the diffusion constant. Moreover, under the same limit procedure, the invariant measure $\mu_k$ and the first passage time of the discrete case converge to their continuous versions. This is true for a general class of Markov chains whose continuum limit leads to a diffusion that is described by a Fokker-Planck equation of the form

$$\frac{\partial P}{\partial t} = \frac{1}{\eta}\frac{\partial}{\partial \epsilon}\left(U'(\epsilon) P\right) + \frac{\Delta}{2\eta}\frac{\partial^2 P}{\partial \epsilon^2}. \tag{54}$$

where $U(\epsilon)$ is an effective trapping potential.

We can now turn the problem around and assume that we have a Markov chain whose evolution is well-approximated by a Fokker-Planck equation of the form (54). Here $U$ is a trapping potential assumed to have a single minimum at $\epsilon = a$ and which diverges sufficiently fast as $|\epsilon| \to \infty$. Then, the invariant measure $\mu(\epsilon)$ is given by

$$\mu(\epsilon) = C e^{-2U(\epsilon)/\Delta}, \tag{55}$$

with $C$ being a normalization constant. In terms of the mesostate models, the invariant measure $\mu(\epsilon)$ prescribes the distribution of the energies $\epsilon$ of mesostates visited under oscillatory shear in the steady-state regime. The absorption region will again be given as $A_\gamma = \{\epsilon > \gamma^2\}$.

The expected waiting time to reach the absorbing region for the first time is then given as [2, 6]

$$\begin{aligned} &\mathbb{E}_a(\tau_{\text{abs}}(\gamma)) \\ &\quad = \frac{2\eta}{\Delta}\int_{-\infty}^{\gamma^2} e^{-2U(y)/\Delta}\left(\int_{\max(a,y)}^{\gamma^2} e^{2U(r)/\Delta}\,\mathrm{d}r\right)\mathrm{d}y. \end{aligned} \tag{56}$$

In the limit that $\Delta$ becomes small, the second integral is dominated by its behavior near $r = \gamma^2$, while the first integral only picks up a dominant contribution near $y = a$. We thus obtain Kramer's formula

$$\mathbb{E}_a(\tau_{\text{abs}}(\gamma)) = \eta\sqrt{\frac{\pi\Delta}{U''(a)}}\,\frac{1}{U'(\gamma^2)}\, e^{2(U(\gamma^2) - U(a))/\Delta}. \tag{57}$$

Note that setting $\eta\Delta = 1$, so that $t = n$, $\Delta = 1/(2\mathcal{N})$ and $U(\epsilon) = (\epsilon - 1/2)^2$, we recover (52).

As in the case of the Ehrenfest model, the phase diagram is determined by $\epsilon_f(\epsilon_0, \gamma^2)$, Eq. (7) of the main text. In particular, the behavior in the metastability regime, $\gamma^2 > \max(a, \epsilon_0)$, now becomes

$$\epsilon_f(\epsilon_0, \gamma) = \gamma^2 - (\gamma^2 - a)\, e^{-\tau/\mathbb{E}_a(\tau_{\rm abs}(\gamma))}. \tag{58}$$

Note that one can use the molecular simulations of [7–9] or the simulations of the stochastic models introduced in [10] to compare with the prediction of (58), which is based on the one dimensional stochastic dynamics given by the Fokker-Planck equation (54), as follows. From the numerical simulations one can extract the steady-state energy distribution, which corresponds to $\mu(\epsilon)$ and furnishes via (55) the effective trapping potential $U(\epsilon)/\Delta$. From the latter $\mathbb{E}_a(\tau_\epsilon)$ can be obtained from (57), providing thereby a prediction for $\epsilon_f(\epsilon_0, \gamma)$, using (58). Note that the functional form of $\epsilon_f(\epsilon_0, \gamma)$ is fully determined, since the overall time scale $\eta$ cancels out. More precisely, $\epsilon_f(\epsilon_0, \gamma)$ is determined by the distribution $\mu(\epsilon)$ of mesostate energies $\epsilon$ at steady-state.

## IV. THE YIELD STRAIN

In this section we obtain the yield strain for the Ehrenfest model. The expected hitting time $\tau_{\rm abs}(\gamma)$ to reach the absorbing state $\epsilon_\gamma = \gamma^2$, given that the system is in the steady-state $\epsilon_{\rm ss} = 1/2 < \epsilon_\gamma$, is given by (52) as

$$\tau_{\rm abs}(\gamma) = 2\sqrt{\pi\mathcal{N}}\,\sqrt{\gamma^2\,(1-\gamma^2)}\,\frac{e^{2\mathcal{N}I(\gamma^2)}}{2\gamma^2 - 1}, \tag{59}$$

where for values of $\gamma^2$ close to $1/2$, we can use the Gaussian approximation for $I$ obtaining thereby

$$\tau_{\rm abs}(\gamma) = \sqrt{\pi\mathcal{N}}\,\frac{e^{4\mathcal{N}\left(\gamma^2-\frac{1}{2}\right)^2}}{2\gamma^2 - 1}. \tag{60}$$

For $\gamma^2 > \max(1/2, \epsilon_0)$, the final energy $\epsilon_f(\epsilon_0, \gamma)$ is then given by Eq. (7) of the main text,

$$\epsilon_f(\epsilon_0, \gamma) = \gamma^2 - \left(\gamma^2 - \frac{1}{2}\right)\, e^{-\tau/\tau_{\rm abs}(\gamma)}, \tag{61}$$

which is independent of $\epsilon_0$, since with almost certainty, the initial state $\epsilon_0$ under cyclic shear quickly relaxes first to the steady-state energy $\epsilon_{\rm ss} = 1/2$, before attempting to reach the absorbing regime.

Following [10], the yield strain $\gamma_y$ is the value of the strain where $\epsilon_f(\epsilon_0, \gamma)$ has a local minimum. Using the Gaussian approximation (60) and making the change of variable

$$\gamma^2 - \frac{1}{2} = \frac{u}{2\sqrt{\mathcal{N}}}, \tag{62}$$

we can rewrite the argument of the exponential in (61) in terms of the rescaled variable $u$ as

$$\frac{\tau}{\tau_{\rm abs}(\gamma)} = \pi^{-\frac{1}{2}}\,\frac{\tau}{\mathcal{N}}\,u e^{-u^2} \equiv \chi w(u), \tag{63}$$

where $\chi = \pi^{-\frac{1}{2}}\,\tau/\mathcal{N}$ is assumed to be large, and

$$w(u) = u e^{-u^2}. \tag{64}$$

Substituting this into (61), we therefore obtain

$$\epsilon_f(u) = \frac{1}{2} + \frac{u}{\sqrt{\mathcal{N}}}\,\left(1 - e^{-\chi w(u)}\right), \tag{65}$$

where $w(u)$ is given by (63). Taking now the derivative of $\epsilon_f(u)$ with respect to $u$ and setting the result to zero, we obtain

$$2\left(u^2 - \frac{1}{2}\right)\,\chi w(u) e^{-\chi w(u)} = 1 - e^{-\chi w(u)}. \tag{66}$$

Note that $u = 0$ is a solution of (66), which is not of interest and moreover leads to a maximum of $\epsilon_f$.

With $\chi$ assumed to be large, the solution we are interested is given by $\chi w(u) \gg 1$ so that $u \gg 1$. In this case, the exponential term on the RHS of (66) can be ignored, and taking logarithms, we obtain

$$\chi w(u) = \ln\left(u^2 - \frac{1}{2}\right) + \ln\left[\chi w(u)\right] + \ln 2. \tag{67}$$

Again, since we are interested in a solution for $\chi w(u) \gg 1$, the last two terms on the RHS give sub-leading order corrections and we are left with

$$\chi w(u) = \ln\left(u^2 - \frac{1}{2}\right). \tag{68}$$

Substituting now (64) for $w(u)$ and taking once more logarithms, we finally obtain

$$u^2 = \ln\chi + \ln u - \ln\ln\left(u^2 - \frac{1}{2}\right). \tag{69}$$

To leading order we thus have $u_0^2 = \ln\chi$, so that

$$u_0 = \sqrt{\ln\left(\pi^{-\frac{1}{2}}\,\frac{\tau}{\mathcal{N}}\right)}. \tag{70}$$

The yield strain $\gamma_y$ follows via (62)

$$\gamma_y^2 = \frac{1}{2}\left(1 + \sqrt{\frac{1}{\mathcal{N}}\,\ln\left(\pi^{-\frac{1}{2}}\,\frac{\tau}{\mathcal{N}}\right)}\right), \tag{71}$$

which is Eq. (8) of the main text.

It turns out that in order to compare the predicted location of the yield strain with the results of the numerical simulations of the Ehrenfest model with $\mathcal{N} = 50$, we need the next order correction to $u_y$. We write $u^2 = u_0^2 + \varepsilon$

and substitute into (69). Expanding the expression to leading order in $\varepsilon$, we obtain

$$u_y = u_0 + \frac{u_0}{2}\,\frac{\ln u_0 - \ln\ln u_0 - \ln 2}{u_0^2 - \frac{1}{2}}. \qquad (72)$$

The gray curves in the inset of Figure 2 of the main paper show the behavior of $-\epsilon_f(\epsilon_0, \gamma^2)$ with $\gamma^2$ in the region near the yield point for different values $\tau$ of the duration of cyclic shearing, $\tau = 10^3, 10^4, \ldots 10^{10}$. The corresponding theoretical predictions for the location of the yield point, as obtained from (72), are indicated by the corresponding circles. As apparent from the figure and the theoretical prediction, the yield strain has a logarithmic dependence on the duration $\tau$ of shearing.

## V. INCORPORATING ADDITIONAL ACTIVATED PROCESSES

So far we have introduced three time scales: The period of the cyclic driving, which we have set to unity, the duration $\tau$ of the applied cyclic shear, and the expected first passage time $\tau_{\mathrm{abs}}(\gamma)$ that governs the transition into the absorbing region $\epsilon \geq \gamma^2$. We found that the yielding transition is characterized by the value of the strain for which the duration of the driving $\tau$ is comparable to the first passage time $\tau_{\mathrm{abs}}(\gamma)$, implying that the yielding transition also depends on the duration $\tau$ of the annealing. For the Ehrenfest model, we obtained a logarithmic dependence on $\tau$, *cf.* (71). In the athermal quasistatic formulation of the Ehrenfest model, once the system reaches a mesostate in the absorbing region it will remain there indefinitely, unless the amplitude of the applied oscillatory shear is increased. The situation is shown in Fig. 1(b) of the main text.

We consider now the effect of adding a further time scale $\tau_{\mathrm{esc}}$ that will mimic a temperature-like activation process. More precisely, this time scale will describe a process by which the system can transition out of a mesostate in side the absorbing region. Such a process could correspond to thermal activation, but it could also be due to some inherent mechanical noise in the system, perhaps inherent to the driving.

In the simplest case the thermal activation process sends the system back from the absorbing state into the steady state, and this happens at a fixed average rate $1/\tau_{\mathrm{esc}}$. This is shown schematically in Fig. 1(c) of the main text. As we will show in Section V A, the introduction of a third time scale $\tau_{\mathrm{esc}}$ implies that when $\tau \gg \tau_{\mathrm{esc}}$, the dynamics is dominated by the interplay of the mechanical relaxation time $\tau_{\mathrm{abs}}(\gamma)$, governing the transition from the steady-state regime into the absorbing region and the thermal relaxation time $\tau_{\mathrm{esc}}$ which triggers a transition back into the steady-state regime. In particular, we will show that these two time scales, $\tau_{\mathrm{abs}}(\gamma)$ and $\tau_{\mathrm{esc}}$, establish the onset of yielding.

More generally, we can extend the dynamics of the Ehrenfest model in the absorption region by allowing thermally activated transitions between mesostates. Let again the mesostate energies be ordered as

$$\epsilon_j = \frac{j}{2\mathcal{N}} \quad j = 0, 1, 2, \ldots 2\mathcal{N}, \qquad (73)$$

so that the energy of the mesostate $\epsilon_j$ when subject to strain $\gamma$ is given as

$$E_j(\gamma) = -\epsilon_j + \frac{\mu}{2}\gamma^2, \qquad (74)$$

for $\gamma^2 \leq \epsilon_j$. Consider an applied oscillatory shear at strain amplitude $\gamma$. We let $k$ denote the smallest integer such that $\epsilon_k \geq \gamma^2$. Starting in the steady-state region $\epsilon_i \approx 1/2$, and with $\gamma^2 > 1/2$, $\epsilon_k$ is the absorbing state that the system will eventually reach under applied cyclic shear at amplitude $\gamma$. In the absence of any relaxation processes or an increase of driving amplitude, the system will remain in this state indefinitely.

Consider now any state $\epsilon_j$ inside the absorption region so that $j \geq k_\gamma$. This state will become mechanically unstable when the strain reaches a magnitude $\sqrt{\epsilon_j}$. Since by definition the applied strain $\gamma^2 \leq \epsilon_j$, there is an energy difference of at least

$$\Delta E_j = \frac{\mu}{2}\left(\epsilon_j - \gamma^2\right). \qquad (75)$$

In other words, $\Delta E_j$ is the difference between the energy at mechanical instability of the mesostate $\epsilon_j$ and the maximum energy attained while driving at strain $\gamma^2$, and for $j \geq k$, *i.e.* inside the absorption region, it is positive. We assume next that $\Delta E_j$ is the relevant energy barrier that needs to be overcome by an activation process and that this happens in an Arrhenius-like fashion, so that the expected activation time is given by

$$\tau_j = \tau_0\, e^{\beta \Delta E_j}. \qquad (76)$$

Here $\tau_0$ is a characteristic holding time and $\beta$ is an inverse effective temperature.

Once an absorbed state becomes activated, the simplest scenario is to assume that the fast mechanical relaxation process takes over and hence a mesostate in state $\epsilon_j$ transits to one of its neighbouring states $\epsilon_{j\pm1}$ with the same transition probabilities $p(\epsilon_j, \epsilon_{j\pm1})$ that characterized the athermal relaxation by cyclic shear. As a result, the activation time now governs the dynamics in the absorbing region. On this time scale, the system can move inside the absorbing region or leave it, once it reaches the mesostate $\epsilon_k$. In the latter case, a fast mechanical relaxation process brings the system into the steady-state regime and the mechanical time scale $\tau_{\mathrm{abs}}(\gamma)$ again dominates the dynamics. The situation is shown schematically in Fig. 1(d) of the main text.

### A. Fixed activation rate

We consider the case when there is a thermal activation process with a fixed rate $1/\tau_{\mathrm{esc}}$ at which the system

transits from the absorbing state $A$ back into the steady-state regime $S$, as shown in Fig. 1(c) of the main text. Denoting by $P_A(t)$ and $P_S(t)$ the probabilities that the system is at time $t$ in state $A$, respectively $S$, given that it was initially in state $S$, the evolution of this pair of probabilities follows a two-state Markov process,

$$\dot{P}_S = -\frac{1}{\tau_{\rm abs}(\gamma)}\, P_S + \frac{1}{\tau_{\rm esc}}\, P_A, \tag{77}$$

$$\dot{P}_A = -\frac{1}{\tau_{\rm esc}}\, P_A + \frac{1}{\tau_{\rm abs}(\gamma)}\, P_S, \tag{78}$$

where $\tau_{\rm abs}(\gamma)$ is given by (52). With the initial condition $P_S(0) = 1$ and $P_A(0) = 0$, the solution is readily found as

$$P_S(t) = 1 - \frac{\tau_{\rm esc}}{\tau_{\rm esc} + \tau_{\rm abs}(\gamma)} \left(1 - e^{-t/\tau_{\rm eff}}\right), \tag{79}$$

$$P_A(t) = \frac{\tau_{\rm esc}}{\tau_{\rm esc} + \tau_{\rm abs}(\gamma)} \left(1 - e^{-t/\tau_{\rm eff}}\right), \tag{80}$$

where

$$\frac{1}{\tau_{\rm eff}} = \frac{1}{\tau_{\rm esc}} + \frac{1}{\tau_{\rm abs}(\gamma)}. \tag{81}$$

Note that when $\tau_{\rm abs}(\gamma) \ll \tau_{\rm esc}$, then at very large times it is very unlikely to find the system in the absorbing state $A$.

Considering a fixed time $\tau$, assuming $\gamma^2 > 1/2.$ and an initial energy $1/2 < \epsilon_0 < \gamma^2$, the system is in the absorbing state $\epsilon = \gamma^2$ with probability $P_A(\tau)$ and in the steady-state $\epsilon = 1/2$ with probability $P_S(t)$, so that in this regime

$$\begin{aligned}\epsilon_f(\epsilon_0, \gamma) =& \frac{1}{2}\, \frac{\tau_{\rm abs}(\gamma)}{\tau_{\rm esc} + \tau_{\rm abs}(\gamma)} \\ &+ \frac{\tau_{\rm esc}}{\tau_{\rm esc} + \tau_{\rm abs}(\gamma)} \left[\gamma^2 - \left(\gamma^2 - \frac{1}{2}\right) e^{-\tau/\tau_{\rm eff}}\right].\end{aligned} \tag{82}$$

Note that when we let $\tau_{\rm esc} \to \infty$, we recover the corresponding expression for the athermal Ehrenfest model,

$$\epsilon_f(\epsilon_0, \gamma) = \gamma^2 - \left(\gamma^2 - \frac{1}{2}\right) e^{-\tau/\tau_{\rm abs}(\gamma)}, \tag{83}$$

as we should.

The inset of Figure 2 of the main text compares the phase diagram of the Ehrenfest model in the absence (gray curves) and presence of a thermal activation process with fixed rate (red curve). In the absence of a thermal activation process the gray curves show the dependence on the duration $\tau$ of applied cyclic shear, $\tau = 10^3, 10^4, \ldots 10^{10}$ (from left to right), as given by (83). The predictions (71) for the yield-strain in the athermal case are indicated by the corresponding gray dots. It is evident that with increasing duration $\tau$ of the applied cyclic shear the yielding transition moves out to larger strain values.

The red curve shows the case when thermal activation processes are present, so that $\epsilon_f(\epsilon_0, \gamma)$ is now given by (82), where $\tau_{\rm esc} = 10^8$ and $\tau = 10^3$. With the introduction of a fixed thermal activation rate, the location of the yielding transition gets pinned at a value that is seen to roughly corresponds to the location of the model without activation, i.e. when $\tau = \tau_{\rm esc}$, implying that $\tau_{\rm esc}$ with the introduction of activation processes $\tau_{\rm esc}$ replaces $\tau$ as the dominant time-scale governing the yielding transition.

To verify these observations, we obtain next from (82) an explicit expression for the yield strain. The calculation is algebraically tedious, but follows the case without activation. We will therefore only sketch out the key steps. We consider again the Gaussian approximation for $\tau_{\rm abs}(\gamma)$, so that *cf.* (63)

$$\frac{\tau}{\tau_{\rm abs}(\gamma)} = \pi^{-\frac{1}{2}}\, \frac{\tau}{\mathcal{N}}\, u e^{-u^2} \equiv \chi w(u), \tag{84}$$

where again $\chi = \pi^{-\frac{1}{2}}\, \tau/\mathcal{N}$ is assumed to be large, and as in the athermal case,

$$w(u) = u e^{-u^2}. \tag{85}$$

Writing the thermal activation time as

$$\frac{\tau}{\tau_{\rm esc}} = \chi\, w_0, \tag{86}$$

so that

$$w_0 = \pi^{\frac{1}{2}}\, \frac{\mathcal{N}}{\tau_{\rm esc}}. \tag{87}$$

The argument of the exponential in (82) then becomes

$$\eta\tau = \chi w_0 + \chi w(u). \tag{88}$$

Taking a derivative of (82) with respect to $u$ and setting the result to zero, leads to

$$\begin{aligned}&\left[1 - \frac{2u^2 - 1}{1 + \frac{u e^{-u^2}}{w_0}}\right] \left(1 - e^{-\chi(w_0 + w(u))}\right) \\ &\quad = 2\chi w(u) \left(u^2 - \frac{1}{2}\right) e^{-\chi(w_0 + w(u))}.\end{aligned} \tag{89}$$

Note that in the limit that $w_0 \to 0$, corresponding to the absence of thermal activation, (89) reduces to (66).

In the limit $\chi \to \infty$ the RHS of (89) goes to zero, so that to this order we must require that the expression on the LHS vanishes, and we obtain

$$1 + \frac{u e^{-u^2}}{w_0} = 2u^2 - 1. \tag{90}$$

From (87) we see that the a large thermal activation time $\tau_{\rm esc}$ implies that $w_0$ is very small, and thus asymptotically we seek a solution of

$$u e^{-u^2} = 2 w_0 \left(u^2 - 1\right). \tag{91}$$

Following steps similar to those of the athermal case, we find

$$u_y^2 = \ln \frac{1}{w_0} - \frac{1}{2} \ln \ln \frac{1}{w_0^4}. \tag{92}$$

The leading order expression for the yield strain $\gamma_y$ is obtained by retaining only the first term in the above expression,

$$\gamma_y^2 = \frac{1}{2} \left( 1 + \sqrt{\frac{1}{\mathcal{N}} \ln \left( \pi^{-\frac{1}{2}} \frac{\tau_{\rm esc}}{\mathcal{N}} \right)} \right), \tag{93}$$

which differs from the corresponding expression (93) for the athermal case by a replacement of the time scale $\tau$ by $\tau_{\rm esc}$.

### B. Barrier height dependent activation rate

We turn next to the case depicted in Fig. 1(d) of the main text, where there is activated dynamics inside the absorbing region. Since the spacing between successive mesostate energies $\epsilon_j$ and $\epsilon_{j+1}$ is assumed to be small, we set $\epsilon_\gamma = \gamma^2$, so that $k/(2\mathcal{N}) = \gamma^2$ and consequently, the absorbing region contains all mesostates $\epsilon_j$ with $j \geq k$, as depicted in Fig. 1(d) of the main text.

Given that the system is in state $j$, the waiting time for activation is assumed to be exponentially distributed with mean $\tau_j$, given by (75) and (76), which becomes

$$\tau_j = \tau_0\, e^{\beta \frac{\mu}{2} (\epsilon_j - \epsilon_k)} \equiv \tau_0\, \eta^{j-k}, \tag{94}$$

where

$$\eta = e^{\frac{\beta\mu}{4\mathcal{N}}}. \tag{95}$$

Thus the steady state mesostate $\epsilon_{\rm ss} = 1/2$ along with the set of absorbing states $\epsilon_j$ for $j \geq k$ constitute a continuous time Markov process with discrete state space, whose transition rates $q(\epsilon, \epsilon')$ are given in terms of the jump probabilities $p(\epsilon_j, \epsilon_{j\pm1})$ of (38) and the holding times as

$$q(\epsilon, \epsilon') = \begin{cases} \tau_{\rm abs}(\gamma)^{-1}, & \epsilon = \epsilon_{\rm ss}, \quad \epsilon' = \epsilon_k, \\ \epsilon_k\, \tau_0^{-1}, & \epsilon = \epsilon_k, \quad \epsilon' = \epsilon_{\rm ss}, \\ \epsilon_j\, \tau_j^{-1}, & \epsilon = \epsilon_j, \quad \epsilon' = \epsilon_{j-1}, \ \ j > k, \\ (1-\epsilon_j)\, \tau_j^{-1}, & \epsilon = \epsilon_j, \quad \epsilon' = \epsilon_{j+1}, \ \ j \geq k. \end{cases} \tag{96}$$

where $\epsilon_j = j/(2\mathcal{N})$, and $\tau_{\rm abs}(\gamma)$ is again the expected first-passage time to the absorbing state $\epsilon_k = \gamma^2$ from the steady state $\epsilon_{\rm ss} = 1/2$, given by (52).

We calculate first the invariant measure $\mu$ of this Markov process. Defining $\mu_{\rm S} = \mu(\epsilon_{\rm ss})$ and $\mu_j = \mu(\epsilon_j)$, and noting that the detailed balance condition holds, the invariant measure satisfies the following sets of equations:

$$\frac{k}{2\mathcal{N}} \frac{\mu_k}{\tau_0} - \frac{\mu_{\rm S}}{\tau_{\rm abs}(\gamma)} = 0, \tag{97}$$

$$\frac{j+1}{2\mathcal{N}} \frac{\mu_{j+1}}{\tau_{j+1}} - \left(1 - \frac{j}{2\mathcal{N}}\right) \frac{\mu_j}{\tau_j} = 0, \quad j \geq k, \tag{98}$$

along with the normalization condition $\mu_{\rm S} + \sum_{j \geq k} \mu_j = 1$. Note that for $j \geq k$ and $\tau_j$ set to unity, the invariant measure for the athermal Ehrenfest model is recovered. With the exponential dependence of $\tau_j$ on $j$, as given by (94), it is readily verified that for $j \geq k$ these recursions are solved in terms of $\mu_k$ as

$$\mu_j = \mu_k\, \eta^{j-k} \frac{\binom{2\mathcal{N}}{j}}{\binom{2\mathcal{N}}{k}}, \tag{99}$$

so that

$$\mu_{\rm S} = \frac{\tau_{\rm abs}(\gamma)}{\tau_0} \frac{k}{2\mathcal{N}} \mu_k. \tag{100}$$

Thus $\mu_k$ is found from the normalization condition as

$$\mu_k = \left[ \frac{\tau_{\rm abs}(\gamma)}{\tau_0} \frac{k}{2\mathcal{N}} + \frac{1}{\binom{2\mathcal{N}}{k}} \sum_{n=0}^{2\mathcal{N}-k} \eta^n \binom{2\mathcal{N}}{k+n} \right]^{-1}. \tag{101}$$

For later use, let us also define the probability $\mu_{\rm A}$ to be in an absorbing state as

$$\mu_{\rm A} = \sum_{j \geq k} \mu_j, \tag{102}$$

so that

$$\mu_{\rm A} = \frac{\mu_k}{\binom{2\mathcal{N}}{k}} \sum_{n=0}^{2\mathcal{N}-k} \eta^n \binom{2\mathcal{N}}{k+n}. \tag{103}$$

In order to proceed, it is convenient to approximate the binomials by Gaussians as in the athermal case, which is a good approximation when $|j - \mathcal{N}| \sim \mathcal{O}(\sqrt{\mathcal{N}})$,

$$\binom{2\mathcal{N}}{j} = \frac{2^{2\mathcal{N}}}{\sqrt{\pi\mathcal{N}}} e^{-4\mathcal{N}\left(\frac{j}{2\mathcal{N}} - \frac{1}{2}\right)^2}. \tag{104}$$

Working out the sum appearing in (101) and (103), we find that

$$\begin{aligned} \frac{\mu_{\rm A}}{\mu_k} &= \frac{1}{\binom{2\mathcal{N}}{k}} \sum_{n=0}^{2\mathcal{N}-k} \eta^n \binom{2\mathcal{N}}{k+n} \\ &= \sum_{n=0}^{2\mathcal{N}-k} e^{\frac{\beta\mu}{4\mathcal{N}}\, n - 4\mathcal{N}\left(\frac{k+n}{2\mathcal{N}} - \frac{1}{2}\right)^2 + 4\mathcal{N}\left(\frac{k}{2\mathcal{N}} - \frac{1}{2}\right)^2}. \end{aligned} \tag{105}$$

The exponent can be simplified by completing squares. Defining

$$\epsilon_{\max} = \frac{\beta\mu}{16\mathcal{N}} + \frac{1}{2}, \tag{106}$$

we obtain

$$\frac{\mu_{\rm A}}{\mu_k} = e^{4\mathcal{N}\left(\epsilon_{\rm max}-\gamma^2\right)^2} \sum_{j=k}^{2\mathcal{N}} e^{-4\mathcal{N}\left(\frac{j}{2\mathcal{N}}-\epsilon_{\rm max}\right)^2}, \qquad (107)$$

which for large $\mathcal{N}$ is well-approximated by an integral, yielding

$$\frac{\mu_{\rm A}}{\mu_k} = 2\mathcal{N}\, e^{4\mathcal{N}\left(\epsilon_{\rm max}-\gamma^2\right)^2} \int_{\gamma^2}^{1} e^{-4\mathcal{N}(\epsilon-\epsilon_{\rm max})^2}\, {\rm d}\epsilon. \qquad (108)$$

For large $N$, the dominant contribution to the integrand comes from values of $\epsilon$ that are close to $\epsilon_{\rm max}$. We therefore need to distinguish three cases: (i) $\epsilon_{\rm max} < \gamma^2$, (ii) $\gamma^2 < \epsilon_{\rm max} < 1$, and (iii) $\epsilon_{\rm max} > 1$. We consider first case (ii), returning to case (i) at the end of this section. Assuming that $\sqrt{\mathcal{N}}(\epsilon_{\rm max} - \gamma^2) \gg 1$, so that the integration limits can be extended to $\pm\infty$ at the cost of introducing exponentially small errors, we obtain

$$\frac{\mu_{\rm A}}{\mu_k} = \sqrt{\pi\mathcal{N}}\, e^{4\mathcal{N}\left(\epsilon_{\rm max}-\gamma^2\right)^2}, \qquad (109)$$

and thus

$$\mu_k = \frac{1}{\frac{\tau_{\rm abs}(\gamma)}{\tau_0}\,\gamma^2 + \sqrt{\pi\mathcal{N}}\, e^{4\mathcal{N}(\epsilon_{\rm max}-\gamma^2)^2}}. \qquad (110)$$

Substituting for $\tau_{\rm abs}(\gamma)$ from (60), this simplifies further as

$$\mu_k = \frac{1}{\sqrt{\pi\mathcal{N}}} \frac{\tau_0}{\frac{\gamma^2}{2\gamma^2-1}\, e^{4\mathcal{N}\left(\gamma^2-\frac{1}{2}\right)^2} + \tau_0\, e^{4\mathcal{N}(\epsilon_{\rm max}-\gamma^2)^2}}, \qquad (111)$$

so that

$$\mu_{\rm S} = \frac{\left(2\gamma^2-1\right)^{-1} e^{4\mathcal{N}\left(\gamma^2-\frac{1}{2}\right)^2}}{\left(2\gamma^2-1\right)^{-1} e^{4\mathcal{N}\left(\gamma^2-\frac{1}{2}\right)^2} + \tau_0\gamma^{-2}\, e^{4\mathcal{N}(\epsilon_{\rm max}-\gamma^2)^2}}. \qquad (112)$$

Recall that the expression for $\tau_{\rm abs}(\gamma)$ is valid only for $\gamma^2 - 1/2 \sim \mathcal{N}^{-1/2}$ and larger. Keeping this in mind, as $\gamma^2$ approaches $1/2$, the $\mu_{\rm S} \to 0$, while in the limit that $\gamma^2$ approaches $\epsilon_{\rm max}$, we have $\mu_{\rm S} \to 1$. Thus as the driving amplitude $\gamma^2$ increases from a value close to $1/2$ to $\epsilon_{\rm max}$, the probability that the system is in the steady-state regime approaches 1.

In fact, defining

$$\tau_{\rm esc}(\gamma) = \sqrt{\pi\mathcal{N}}\,\frac{\tau_0}{\gamma^2}\, e^{4\mathcal{N}\left(\epsilon_{\rm max}-\gamma^2\right)^2}, \qquad (113)$$

we can rewrite $\mu_{\rm A}$ and $\mu_{\rm S}$ as

$$\mu_{\rm A} = \frac{\tau_{\rm esc}(\gamma)}{\tau_{\rm abs}(\gamma) + \tau_{\rm esc}(\gamma)} \qquad (114)$$

$$\mu_{\rm S} = \frac{\tau_{\rm abs}(\gamma)}{\tau_{\rm abs}(\gamma) + \tau_{\rm esc}(\gamma)}, \qquad (115)$$

where $\tau_{\rm abs}(\gamma)$ is, as before, the mechanical relaxation time from steady-state into the absorbing region

$$\tau_{\rm abs}(\gamma) = \sqrt{\pi\mathcal{N}}\, \left(2\gamma^2-1\right)^{-1} e^{4\mathcal{N}\left(\gamma^2-\frac{1}{2}\right)^2}. \qquad (116)$$

Comparing (114) and (115) with the corresponding asymptotic expression (79) in the case of a fixed thermal activation time, we see that $\tau_{\rm esc}(\gamma)$, as given by (113), is the characteristic thermal relaxation time from the absorbing region into the steady state regime.

We have reduced the dynamics between absorbing and steady state region to a two-state continuous-time Markov process, as in Fig. 1(c) of the main text, with both the absorption and escape rate depending on $\gamma$.

The corresponding calculation for the case (i) where $\epsilon_{\rm max} < \gamma^2$ implies that the integral in (108) is dominated by the values near $\epsilon = \gamma^2$, yielding asymptotically in $\mathcal{N}$

$$\frac{\mu_{\rm A}}{\mu_k} = \frac{1}{2}\,\frac{1}{\gamma^2 - \epsilon_{\rm max}}, \qquad (117)$$

so that

$$\tau_{\rm esc}(\gamma) = \frac{\tau_0}{2}\,\frac{1}{\gamma^2(\gamma^2 - \epsilon_{\rm max})}. \qquad (118)$$


[1] A. Bovier, M. Eckhoff, V. Gayrard, and M. Klein, Probability Theory and Related Fields **119**, 99 (2001).

[2] A. Bovier and F. den Hollander, *Metastability* (Springer-Verlag, New York, 2016).

[3] J. R. Norris, *Markov chains* (Cambridge university press, Cambridge, 1998).

[4] R. Bellman and T. E. Harris, Pacific Journal of Mathematics **1**, 179 (1951).

[5] M. Kac, The American Mathematical Monthly **54**, 369 (1947).

[6] N. G. Van Kampen, *Stochastic processes in physics and chemistry* (Elsevier, Amsterdam, 1992).

[7] H. Bhaumik, G. Foffi, and S. Sastry, Proceedings of the National Academy of Sciences (USA) **118**, e2100227118 (2021).

[8] W.-T. Yeh, M. Ozawa, K. Miyazaki, T. Kawasaki, and L. Berthier, Physical review letters **124**, 225502 (2020).

[9] C. Liu, E. E. Ferrero, E. A. Jagla, K. Martens, A. Rosso, and L. Talon, arXiv preprint arXiv:2012.15310 (2020).

[10] S. Sastry, Phys. Rev. Lett. **126**, 255501 (2021).
